# Supplementary material for: Excitations and benchmark ensemble density functional theory for two electrons
Source: arXiv:1402.5444 ancillary file (2014-02-25)
Supplement: Supplementary file 1 [file ensJCP_SuppMatl.pdf]

# Excitations and benchmark ensemble density functional theory for two electrons: Supplemental Material

Aurora Pribram-Jones,[1] Zeng-hui Yang,[2] John Trail,[3] Kieron Burke,[1] Richard J. Needs,[3] and Carsten A. Ullrich[2]
[1)] *Department of Chemistry, University of California-Irvine, Irvine, CA 92697, USA*
[2)] *Department of Physics and Astronomy, University of Missouri, Columbia, MO 65211, USA*
[3)] *Theory of Condensed Matter Group, Cavendish Laboratory, University of Cambridge, Cambridge CB3 0HE, United Kingdom*

(Dated: 21 February 2014)

Numerical details, additional data, extended tables, and supplemental figures.

PACS numbers: 31.10.+z, 31.15.E-, 31.15.ee, 71.15.Qe

## I. DISCRETIZATION SCHEMES

Using 1D systems as an example, the first scheme we tested is

$$-\frac{1}{2}\frac{d^2\phi(x)}{dx^2} \approx \frac{\phi(x_i)}{(x_i - x_{i-1})(x_{i+1} - x_i)} - \frac{\phi(x_{i-1})}{(x_i - x_{i-1})(x_{i+1} - x_{i-1})} - \frac{\phi(x_{i+1})}{(x_{i+1} - x_i)(x_{i+1} - x_{i-1})}. \tag{1}$$

The second scheme is derived following Ref. 1, where

$$-\frac{1}{2}\frac{d^2\phi(x)}{dx^2} \approx \frac{\phi(x_i)}{4}\left\{\frac{1}{(x_{i+1} - x_i)^2}\left[1 + \frac{x_{i+2} - x_i}{x_{i+1} - x_{i-1}}\right] + \frac{1}{(x_i - x_{i-1})^2}\left[1 + \frac{x_i - x_{i-2}}{x_{i+1} - x_{i-1}}\right]\right\} - \frac{\phi(x_{i-1})}{4(x_i - x_{i-1})^2}\left[\sqrt{\frac{x_i - x_{i-2}}{x_{i+1} - x_{i-1}}} + \sqrt{\frac{x_{i+1} - x_{i-1}}{x_i - x_{i-2}}}\right] - \frac{\phi(x_{i+1})}{4(x_{i+1} - x_i)^2}\left[\sqrt{\frac{x_{i+1} - x_{i-1}}{x_{i+2} - x_i}} + \sqrt{\frac{x_{i+2} - x_i}{x_{i+1} - x_{i-1}}}\right]. \tag{2}$$

On a uniform grid, both discretization schemes reduce to the same form, and the error is on the order of $(x_i - x_{i-1})^2 d^4\phi(x)/dx^4$. On a nonuniform grid, Eq. (2) has smaller systematic error because its Hamiltonian matrix stays hermitian and simplifies diagonalization. On the other hand, the leading term of the inherent error of the discretization for Eq. (1) is

$$-\frac{h^2}{24}\frac{d^4\phi(x)}{dx^4} - \frac{a}{6}\frac{d^3\phi(x)}{dx^3}, \tag{3}$$

and that for Eq. (2) is

$$\left(-\frac{ab}{32h^4} - \frac{5ac}{16h^4} + \frac{-a+b+c}{8h^3}\right)\phi(x), \tag{4}$$

where $h = x_i - x_{i-1}$, $a = x_{i+1} - 2x_i + x_{i-1}$, $b = -x_{i-2} + 2x_{i-1} - x_i$, $c = x_{i+2} - x_{i+1} - x_i + x_{i-1}$. The error (4) is larger than the error (3) in general.

Eqs. (1) and (2) were tested on all the systems studied in this paper. We find that both work well for the 1D box, but for atomic systems, Eq. (2) incurs noticable errors near $r = 0$ in the density. This error propagates, producing artificial dips in $v_{\rm XC}$. We also find the error in the density near $r = 0$ using Eq. (1) is larger than the error at other grid points, but is still orders of magnitude smaller than that of Eq. (2). All the results presented in this paper have therefore been obtained using Eq. (1).

## II. 1D FLAT BOX ENSEMBLES

The first excited state of the box is a triplet state, so the calculation of $E_{\rm HX}$ needs to reflect the triplet nature of the first excited states:

$$E_{\rm HX} = (1-3\mathtt{w})\left\langle \Psi_{s,0}\middle|\hat{V}_{\rm ee}\middle|\Psi_{s,0}\right\rangle + w\sum_{i=1}^{3}\left\langle \Psi_{s,i}\middle|\hat{V}_{\rm ee}\middle|\Psi_{s,i}\right\rangle, \tag{5}$$

where the multi-determinant wavefunctions are

$$\Psi_{s,1}(\mathbf{r},\mathbf{r}') = \frac{1}{2}\begin{vmatrix}\phi_{1\uparrow}(\mathbf{r}) & \phi_{2\downarrow}(\mathbf{r})\\ \phi_{1\uparrow}(\mathbf{r}') & \phi_{2\downarrow}(\mathbf{r}')\end{vmatrix} + \frac{1}{2}\begin{vmatrix}\phi_{1\downarrow}(\mathbf{r}) & \phi_{2\uparrow}(\mathbf{r})\\ \phi_{1\downarrow}(\mathbf{r}') & \phi_{2\uparrow}(\mathbf{r}')\end{vmatrix},$$
$$\Psi_{s,2}(\mathbf{r},\mathbf{r}') = \frac{1}{\sqrt{2}}\begin{vmatrix}\phi_{1\uparrow}(\mathbf{r}) & \phi_{2\uparrow}(\mathbf{r})\\ \phi_{1\uparrow}(\mathbf{r}') & \phi_{2\uparrow}(\mathbf{r}')\end{vmatrix},$$
$$\Psi_{s,3}(\mathbf{r},\mathbf{r}') = \frac{1}{\sqrt{2}}\begin{vmatrix}\phi_{1\downarrow}(\mathbf{r}) & \phi_{2\downarrow}(\mathbf{r})\\ \phi_{1\downarrow}(\mathbf{r}') & \phi_{2\downarrow}(\mathbf{r}')\end{vmatrix}. \tag{6}$$

Using this scheme, Table I shows calculated excitation energies for various $\mathtt{w}$-values with high accuracy, including a double excitation energy. In Table II, we calculate energy components, which satisfy the exact conditions derived in the body of the paper and show the strong $\mathtt{w}$-dependence of these quantities.

Exact ensemble densities (Fig. 1) and KS potentials (2) for the 1d box show that the bump up in the potentials near the center of the box are needed to ensure that the ensemble KS densities have characteristics of the excited states, with larger bumps corresponding to higher proportions of the excited states in the ensembles.

| 2-multiplet ensemble: $E_1 - E_0 = 12.4399$ Hartree | | | | | | | | |
|---|---|---|---|---|---|---|---|---|
| $\mathtt{w}_2$ | 0.25 | 0.21875 | 0.1875 | 0.15625 | 0.125 | 0.09375 | 0.0625 | 0.03125 |
| $E^{\rm KS}_{1,\mathtt{w}_2} - E^{\rm KS}_{0,\mathtt{w}_2}$ | 13.9402 | 13.9367 | 13.9322 | 13.9267 | 13.9201 | 13.9125 | 13.9036 | 13.8932 |
| $\partial E_{{\rm xc},\mathtt{w}_2}[I=2,n]/\partial \mathtt{w}_2\vert_{n=n_{\mathtt{w}_2}}$ | -4.5010 | -4.4905 | -4.4769 | -4.4604 | -4.4407 | -4.4178 | -4.3910 | -4.3598 |
| $(E_1 - E_0)_{\mathtt{w}_2}$ | 12.4399 | 12.4399 | 12.4399 | 12.4399 | 12.4399 | 12.4399 | 12.4399 | 12.4399 |
| 3-multiplet ensemble: $E_2 - E_0 = 15.6202$ Hartree | | | | | | | | |
| $\mathtt{w}_3$ | 0.2 | 0.175 | 0.15 | 0.125 | 0.1 | 0.075 | 0.05 | 0.025 |
| $E^{\rm KS}_{2,\mathtt{w}_3} - E^{\rm KS}_{0,\mathtt{w}_3}$ | 14.2179 | 14.1817 | 14.1460 | 14.1106 | 14.0757 | 14.0412 | 14.0072 | 13.9735 |
| $\partial E_{{\rm xc},\mathtt{w}_3}[I=3,n]/\partial \mathtt{w}_3\vert_{n=n_{\mathtt{w}_3}}$ | 2.7358 | 2.7448 | 2.7538 | 2.7626 | 2.7713 | 2.7799 | 2.7884 | 2.7969 |
| $(E_2 - E_0)_{\mathtt{w}_2,\mathtt{w}_3}$ | 15.6202 | 15.6202 | 15.6202 | 15.6202 | 15.6201 | 15.6201 | 15.6201 | 15.6202 |
| 4-multiplet ensemble: $E_3 - E_0 = 28.8561$ Hartree (double-excitation) | | | | | | | | |
| $\mathtt{w}_4$ | 0.166666 | 0.145833 | 0.125 | 0.104166 | 0.083333 | 0.0625 | 0.041666 | 0.020833 |
| $E^{\rm KS}_{3,\mathtt{w}_4} - E^{\rm KS}_{0,\mathtt{w}_4}$ | 28.7534 | 28.7081 | 28.6646 | 28.6228 | 28.5826 | 28.5439 | 28.5066 | 28.4706 |
| $\partial E_{{\rm xc},\mathtt{w}_4}[I=4,n]/\partial \mathtt{w}_4\vert_{n=n_{\mathtt{w}_4}}$ | 1.1061 | 1.0433 | 1.0694 | 1.0945 | 1.1186 | 1.1418 | 1.1642 | 1.1858 |
| $(E_3 - E_0)_{\mathtt{w}_2,\mathtt{w}_3,\mathtt{w}_4}$ | 28.8561 | 28.8561 | 28.8561 | 28.8561 | 28.8561 | 28.8561 | 28.8561 | 28.8561 |
| 5-multiplet ensemble: $E_4 - E_0 = 37.7028$ Hartree | | | | | | | | |
| $\mathtt{w}_5$ | 0.111111 | 0.097222 | 0.083333 | 0.069444 | 0.055555 | 0.041666 | 0.027777 | 0.013888 |
| $E^{\rm KS}_{4,\mathtt{w}_5} - E^{\rm KS}_{0,\mathtt{w}_5}$ | 38.8375 | 38.8436 | 38.8494 | 38.8550 | 38.8602 | 38.8652 | 38.8700 | 38.8746 |
| $\partial E_{{\rm xc},\mathtt{w}_5}[I=5,n]/\partial \mathtt{w}_5\vert_{n=n_{\mathtt{w}_5}}$ | -1.1279 | -1.1529 | -1.1766 | -1.1991 | -1.2205 | -1.2408 | -1.2602 | -1.2787 |
| $(E_4 - E_0)_{\mathtt{w}_2,\mathtt{w}_3,\mathtt{w}_4,\mathtt{w}_5}$ | 37.7028 | 37.7028 | 37.7028 | 37.7027 | 37.7027 | 37.7027 | 37.7027 | 37.7028 |

TABLE I. Excitation energies of the 1D box calculated at different $\mathtt{w}$ values using the exact ensemble KS systems. All energies are in Hartree. Accurate excitation energies are extracted for all values of $\mathtt{w}$ and $M$ tested, including a double excitation.

| $\mathtt{w}$ | 0.25 | 0.21875 | 0.1875 | 0.15625 | 0.125 | 0.09375 | 0.0625 | 0.03125 |
|---|---|---|---|---|---|---|---|---|
| $E_{\mathtt{w}}$ | 24.4525 | 23.2862 | 22.1200 | 20.9537 | 19.7875 | 18.6213 | 17.4550 | 16.2888 |
| $T_{\rm S}$ | 21.0032 | 19.6171 | 18.2310 | 16.8450 | 15.4590 | 14.0730 | 12.6871 | 11.3013 |
| $E_{\rm H}$ | 9.7265 | 9.8134 | 9.9084 | 10.0116 | 10.1230 | 10.2425 | 10.3702 | 10.5061 |
| $E_{\rm XC}$ | -6.2773 | -6.1443 | -6.0195 | -5.9029 | -5.7945 | -5.6943 | -5.6023 | -5.5186 |
| $E_{\rm HX}$ | 4.3150 | 4.4414 | 4.5678 | 4.6942 | 4.8205 | 4.9467 | 5.0729 | 5.1990 |
| $E_{\rm X}$ | -5.4115 | -5.3720 | -5.3406 | -5.3175 | -5.3025 | -5.2958 | -5.2973 | -5.3070 |
| $E_{\rm C}$ | -0.8658 | -0.7723 | -0.6788 | -0.5854 | -0.4919 | -0.3985 | -0.3050 | -0.2116 |
| $T_{\rm C}$ | 0.0320 | 0.0422 | 0.0523 | 0.0623 | 0.0724 | 0.0823 | 0.0923 | 0.1021 |
| $V_{\rm C}$ | -0.8978 | -0.8145 | -0.7311 | -0.6477 | -0.5643 | -0.4808 | -0.3973 | -0.3137 |

TABLE II. Energy decomposition of the two-multiplet ensemble of the 1D box at different $\mathtt{w}$ values. All energies are in Hartree. The Hartree and exchange energies are defined with respect to the soft-Coulomb interaction in Eq. (78). Listed $E_{\rm H}$ values are that of $E_{\rm H}^{\rm trad}$, and listed $E_{\rm XC}$ values are compatible with that.

## III. CHARGE-TRANSFER EXCITATION WITH 1D BOX

Charge-transfer excitations are notoriously difficult, as described in the main text. Here, using a charge-transfer 1d box model, we show that ensemble DFT has no difficulty extracting charge-transfer excitation energies.

## IV. HOOKE'S ATOM

Figures 3 and 4 demonstrate how little densities and potentials for the Hooke's atom ensemble change with $\mathtt{w}$. In addition, the numerical difficulties near $r = 0$ are obvious in the potential. Despite these differences from the other examples, extracted excitation energies remain highly accurate.

## V. HELIUM ENSEMBLES: STRICTLY SINGLET, MIXED SYMMETRY, AND STRICTLY TRIPLET

Helium's multiplet structure allows us to build a variety of ensembles from the first few excited states. This allows us to test the symmetry projected ensembles for singlets and triplets, as well as mixed symmetry bi-ensembles and ensembles of mixed symmetry and multiple excited states. The 2-multiplet ensemble is constructed of the singlet ground state and the triplet first

| $3\mathtt{w}$ | 0.5 | 0.4 | 0.3 | 0.2 | 0.1 | 0.08 | 0.06 | 0.04 | 0.02 |
|---|---|---|---|---|---|---|---|---|---|
| $E^{\rm KS}_{1,\mathtt{w}} - E^{\rm KS}_{0,\mathtt{w}}$ | 2.2048 | 2.2678 | 2.3221 | 2.3692 | 2.4092 | 2.4161 | 2.4225 | 2.4280 | 2.4317 |
| $1/3\partial E_{\rm xc,\mathtt{w}}[n]/\partial n\|_{n=n_\mathtt{w}}$ | 0.1993 | 0.1287 | 0.0748 | 0.0299 | -0.0108 | -0.0178 | -0.0242 | -0.0297 | -0.0334 |
| $(E_1 - E_0)_\mathtt{w}$ | 2.4042 | 2.3965 | 2.3970 | 2.3990 | 2.3983 | 2.3983 | 2.3983 | 2.3983 | 2.3983 |
| $E_\mathtt{w}$ | 139.453 | 139.214 | 138.974 | 138.734 | 138.494 | 138.446 | 138.398 | 138.350 | 138.302 |
| $T_{\rm S}$ | 82.6734 | 77.0316 | 71.4367 | 65.8806 | 60.3570 | 59.2558 | 58.1556 | 57.0564 | 55.9582 |
| $E_{\rm H}$ | 127.587 | 133.429 | 141.199 | 150.897 | 162.523 | 165.080 | 167.714 | 170.425 | 173.213 |
| $V$ | 12.0170 | 11.1226 | 10.2281 | 9.3337 | 8.4393 | 8.2604 | 8.0815 | 7.9026 | 7.7237 |
| $E_{\rm XC}$ | -82.8238 | -82.3694 | -83.8900 | -87.3775 | -92.8258 | -94.1503 | -95.5529 | -97.0338 | -98.5927 |
| $E_{\rm HX}$ | 51.2492 | 58.7052 | 66.1011 | 73.4495 | 80.7598 | 82.2179 | 83.6749 | 85.1307 | 86.5854 |
| $E_{\rm X}$ | -76.3375 | -74.7235 | -75.0977 | -77.4475 | -81.7637 | -82.8622 | -84.0391 | -85.2942 | -86.6275 |
| $E_{\rm C}$ | -6.4863 | -7.6459 | -8.7923 | -9.9300 | -11.0621 | -11.2880 | -11.5139 | -11.7396 | -11.9652 |
| $T_{\rm C}$ | 5.1280 | 5.9018 | 6.6288 | 7.3170 | 7.9726 | 8.1003 | 8.2269 | 8.3525 | 8.4770 |
| $V_{\rm C}$ | -11.6142 | -13.5477 | -15.4211 | -17.2470 | -19.0347 | -19.3883 | -19.7407 | -20.0920 | -20.4422 |

TABLE III. First excitation energy and energy decomposition of the two-multiplet ensemble of the 1D charge-transfer box at different $\mathtt{w}$ values. All energies are in eV. Exact first excitation energy $E_1 - E_0 = 2.3983$ eV. The Hartree and exchange energies are defined with respect to the soft-Coulomb interaction in Eq. (78). Listed $E_{\rm H}$ values are that of $E_{\rm H}^{\rm trad}$, and listed $E_{\rm XC}$ values are compatible with that.

| w | 0.5 | 0.4 | 0.3 | 0.2 | 0.1 | 0.08 | 0.06 | 0.04 | 0.02 |
|---|---|---|---|---|---|---|---|---|---|
| $\epsilon_2^{(\mathtt{w})} - \epsilon_1^{(\mathtt{w})}$ | 11.774 | 11.713 | 11.653 | 11.595 | 11.536 | 11.524 | 11.512 | 11.499 | 11.487 |
| $\partial E_{\rm XC}[w,n]/\partial w\|_{n=n^{(\mathtt{w})}}$ | -1.988 | -1.927 | -1.868 | -1.809 | -1.750 | -1.738 | -1.726 | -1.714 | -1.701 |
| $\omega$ | 9.786 | 9.786 | 9.786 | 9.786 | 9.786 | 9.786 | 9.786 | 9.786 | 9.786 |
| Relative error | $8\times10^{-6}$ | $-3\times10^{-6}$ | $-3\times10^{-6}$ | $5\times10^{-6}$ | $-7\times10^{-8}$ | $-2\times10^{-7}$ | $-2\times10^{-7}$ | $-6\times10^{-8}$ | $-5\times10^{-7}$ |
| $E_\mathtt{w}$ | 59.310 | 58.331 | 57.353 | 56.374 | 55.396 | 55.200 | 55.004 | 54.808 | 54.613 |
| $T$ | 21.564 | 20.864 | 20.164 | 19.465 | 18.765 | 18.625 | 18.485 | 18.345 | 18.205 |
| $T_{\rm S}$ | 21.084 | 20.323 | 19.563 | 18.804 | 18.046 | 17.894 | 17.743 | 17.592 | 17.440 |
| $E_{\rm XC}$ | -15.156 | -15.123 | -15.097 | -15.079 | -15.069 | -15.068 | -15.068 | -15.067 | -15.067 |
| $E_{\rm HX}$ | 12.733 | 12.993 | 13.252 | 13.508 | 13.763 | 13.813 | 13.864 | 13.914 | 13.965 |
| $E_{\rm H}$ | 26.424 | 26.732 | 27.047 | 27.370 | 27.698 | 27.765 | 27.832 | 27.899 | 27.967 |
| $E_{\rm X}$ | -13.690 | -13.739 | -13.796 | -13.861 | -13.936 | -13.952 | -13.968 | -13.985 | -14.002 |
| $E_{\rm C}$ | -1.466 | -1.384 | -1.301 | -1.218 | -1.134 | -1.116 | -1.100 | -1.082 | -1.066 |
| $T_{\rm C}$ | 0.480 | 0.541 | 0.602 | 0.661 | 0.719 | 0.731 | 0.742 | 0.754 | 0.765 |
| $T_{\rm C}^{\rm virial}$ | 0.496 | 0.557 | 0.617 | 0.676 | 0.734 | 0.746 | 0.757 | 0.769 | 0.780 |
| $V_{\rm C}$ | -1.945 | -1.925 | -1.903 | -1.879 | -1.853 | -1.847 | -1.842 | -1.836 | -1.830 |

TABLE IV. First excitation energy and energy decomposition of the Hooke's atom at different $\mathtt{w}$ values. All energies are in eV. $T = -E + 3V_{\rm ext}$ according to the virial theorem for Hooke's atom with interacting electrons. The xc virial theorem still holds, but due to the numerical convergence problem of $v_{\rm XC}$, the error is bigger than those of the helium atom.

excited state. The 3-multiplet ensemble includes ground, triplet first excited, and singlet second excited states. The singlet ensemble, the focus of our previous work, is built from the ground and second excited states. Finally, a triplet ensemble is constructed from the triplet 1s2s first excited state and the triplet 1s3s excited state.

### A. Singlet Helium Ensemble

Table VII shows the variation in exchange and exchange-correlation energy components with $\mathtt{w}$ for the approximations analyzed in the main text. None of these approximations produce exchange-correlation potentials with the bumps recovered by our work's symmetry-eigenstate Hartree-exchange (SEHX) approximation.

### B. Singlet-Triplet Helium Ensemble

### C. Singlet-triplet-singlet ensemble

The singlet-triplet-singlet ensemble allows us to compare excitation energies extracting for the second excited state in two different ensembles: the singlet ensemble and

| 2-multiplet ensemble: $E_1 - E_0 = 19.8231 eV$ | | | | | | | | |
|---|---|---|---|---|---|---|---|---|
| $\mathtt{w}_2$ | 0.25 | 0.21875 | 0.1875 | 0.15625 | 0.125 | 0.09375 | 0.0625 | 0.03125 |
| $E^{\rm KS}_{1,\mathtt{w}_2} - E^{\rm KS}_{0,\mathtt{w}_2}$ | 25.1035 | 24.0231 | 23.3161 | 22.8269 | 22.4676 | 22.1832 | 21.9303 | 21.6502 |
| $\partial E_{{\rm xc},\mathtt{w}_2}[n]/\partial \mathtt{w}_2\|_{n=n_{\mathtt{w}_2}}$ | -15.8099 | -12.6093 | -10.4842 | -9.0146 | -7.9358 | -7.0819 | -6.3458 | -5.4351 |
| $(E_1 - E_0)_{\mathtt{w}_2}$ | 19.8336 | 19.8200 | 19.8213 | 19.8220 | 19.8224 | 19.8226 | 19.8150 | 19.8385 |
| 3-multiplet ensemble: $E_2 - E_0 = 20.6191 eV$ | | | | | | | | |
| $\mathtt{w}_3$ | 0.2 | 0.175 | 0.15 | 0.125 | 0.1 | 0.075 | 0.05 | 0.025 |
| $E^{\rm KS}_{2,\mathtt{w}_3} - E^{\rm KS}_{0,\mathtt{w}_3}$ | 26.8457 | 26.5886 | 26.3440 | 26.1112 | 25.8895 | 25.6783 | 25.4770 | 25.2853 |
| $\partial E_{{\rm xc},\mathtt{w}_3}[n]/\partial \mathtt{w}_3\|_{n=n_{\mathtt{w}_3}}$ | -0.9596 | -0.8954 | -0.8342 | -0.7761 | -0.7207 | -0.6680 | -0.6176 | -0.5696 |
| $(E_2 - E_0)_{\mathtt{w}_2,\mathtt{w}_3}$ | 20.6270 | 20.6168 | 20.6178 | 20.6182 | 20.6184 | 20.6185 | 20.6129 | 20.6306 |

TABLE V. Excitation energies of the helium atom at different $\mathtt{w}$ values using the exact ensemble KS systems. All energies are in eV.

| $\mathtt{w}$ | 0.5 | 0.4 | 0.3 | 0.2 | 0.1 | 0.08 | 0.06 | 0.04 | 0.02 |
|---|---|---|---|---|---|---|---|---|---|
| $E_{\mathtt{w}}$ | -68.70 | -70.76 | -72.83 | -74.89 | -76.95 | -77.36 | -77.78 | -78.19 | -78.60 |
| $T$ | 68.70 | 70.76 | 72.83 | 74.89 | 76.95 | 77.36 | 77.78 | 78.19 | 78.60 |
| $T_{\rm S}$ | 67.74 | 69.75 | 71.79 | 73.84 | 75.92 | 76.33 | 76.75 | 77.17 | 77.58 |
| $V_{\rm ext}$ | -153.66 | -159.68 | -165.70 | -171.72 | -177.73 | -178.94 | -180.14 | -181.34 | -182.55 |
| $E_{\rm XC}$ | -21.86 | -22.96 | -24.23 | -25.66 | -27.26 | -27.60 | -27.94 | -28.30 | -28.65 |
| $E_{\rm HX}$ | 18.36 | 20.37 | 22.31 | 24.21 | 26.06 | 26.42 | 26.79 | 27.15 | 27.51 |
| $E_{\rm H}$ | 39.09 | 42.13 | 45.32 | 48.65 | 52.13 | 52.84 | 53.56 | 54.29 | 55.02 |
| $E_{\rm X}$ | -20.73 | -21.76 | -23.00 | -24.44 | -26.07 | -26.42 | -26.77 | -27.14 | -27.50 |
| $E_{\rm C}$ | -1.134 | -1.200 | -1.226 | -1.220 | -1.189 | -1.180 | -1.171 | -1.161 | -1.150 |
| $T_{\rm C}$ | 0.965 | 1.016 | 1.041 | 1.046 | 1.034 | 1.030 | 1.026 | 1.021 | 1.015 |
| $T_{\rm C}^{\rm virial}$ | 0.963 | 1.014 | 1.039 | 1.044 | 1.032 | 1.028 | 1.023 | 1.018 | 1.013 |
| $V_{\rm C}$ | -2.100 | -2.216 | -2.267 | -2.266 | -2.223 | -2.211 | -2.196 | -2.182 | -2.165 |

TABLE VI. Exact ensemble energy components of the singlet ensemble of helium atom. All the energies are in eV. $T = -E$ according to the virial theorem for atoms. $E_{\rm H}$ is defined in Eq. (29). $T_{\rm C}^{\rm virial}$ is obtained by the virial theorem Eq. (62). The differences between $T_{\rm C}$'s and $T_{\rm C}^{\rm virial}$'s are due to numerical errors.

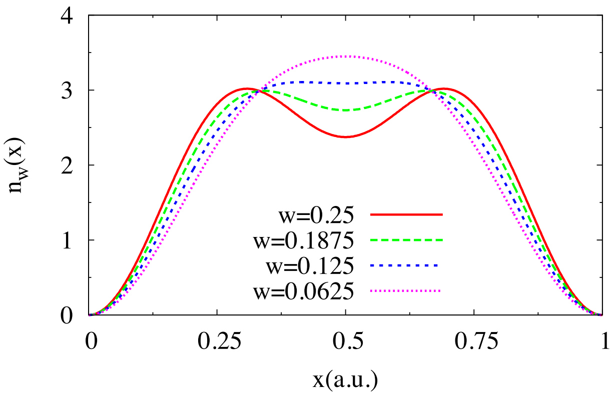


FIG. 1. Exact ensemble densities of the 1D box with two electrons. The ensemble contains the ground state and the first (triplet) excited state.

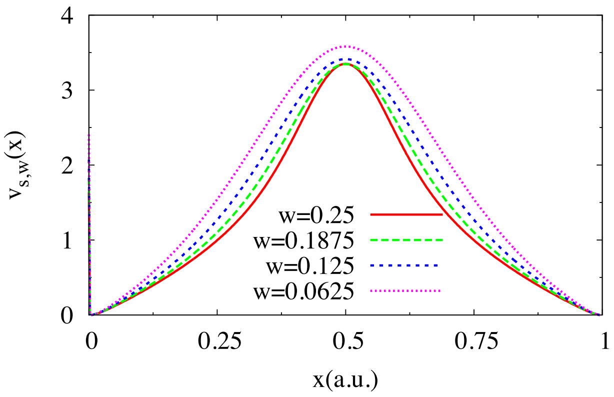


FIG. 2. Exact ensemble KS potentials of the 1D box with two electrons. The ensemble contains the ground state and the first (triplet) excited state.

the 3-multiplet ensemble shown below. The incredibly accurate results given in our previous work, compared to those of the main text, show that symmetry projection can provide more accurate calculations of excitation energies.

| w | 0.5 | 0.4 | 0.3 | 0.2 | 0.1 | 0.08 | 0.06 | 0.04 | 0.02 |
|---|---|---|---|---|---|---|---|---|---|
| $E_{\mathrm{XC}}^{\mathrm{qLDA}}$ | -20.96 | -22.10 | -23.28 | -24.50 | -25.76 | -26.02 | -26.28 | -26.54 | -26.81 |
| $E_{\mathrm{X}}^{\mathrm{Nagy}}$ | -19.39 | -20.46 | -21.85 | -23.55 | -25.56 | -26.00 | -26.45 | -26.92 | -27.39 |
| $E_{\mathrm{X}}^{\mathrm{EXX}}$ | -20.91 | -21.91 | -23.12 | -24.52 | -26.11 | -26.45 | -26.80 | -27.15 | -27.51 |
| $G_{\mathrm{H}}$ | 1.604 | 1.547 | 1.359 | 1.039 | 0.587 | 0.481 | 0.369 | 0.252 | 0.129 |
| $G_{\mathrm{X}}$ | -0.090 | -0.093 | -0.086 | -0.069 | -0.041 | -0.034 | -0.026 | -0.018 | -0.009 |

TABLE VII. qLDA and EXX energy components of the singlet ensemble of helium atom. $G_{\mathrm{H}}$ and $G_{\mathrm{X}}$ are the ghost terms in $E_{\mathrm{H}}$ and $E_{\mathrm{X}}^{\mathrm{Nagy}}$, respectively.

| w | 0.25 | 0.21875 | 0.1875 | 0.15625 | 0.125 | 0.09375 | 0.0625 | 0.03125 |
|---|---|---|---|---|---|---|---|---|
| $E_{1,\mathtt{w}}^{\mathrm{KS}} - E_{0,\mathtt{w}}^{\mathrm{KS}}$ | 25.1035 | 24.0231 | 23.3161 | 22.8269 | 22.4676 | 22.1832 | 21.9303 | 21.6502 |
| $\partial E_{\mathrm{xc},\mathtt{w}}[n]/\partial w\|_{n=n_{\mathtt{w}}}$ | -15.8099 | -12.6093 | -10.4842 | -9.0146 | -7.9358 | -7.0819 | -6.3458 | -5.4351 |
| $(E_1 - E_0)_{\mathtt{w}}$ | 19.8336 | 19.8200 | 19.8213 | 19.8220 | 19.8224 | 19.8226 | 19.8150 | 19.8385 |
| $E_{\mathtt{w}}$ | -64.1459 | -66.0043 | -67.8628 | -69.7212 | -71.5796 | -73.4380 | -75.2964 | -77.1548 |
| $T_{\mathrm{S}}$ | 63.5171 | 65.2586 | 67.0297 | 68.8232 | 70.6343 | 72.4595 | 74.2966 | 76.1437 |
| $E_{\mathrm{H}}$ | 33.3604 | 35.7433 | 38.2452 | 40.8662 | 43.6061 | 46.4652 | 49.4432 | 52.5403 |
| $V$ | -140.190 | -145.635 | -151.080 | -156.525 | -161.970 | -167.416 | -172.861 | -178.306 |
| $E_{\mathrm{XC}}$ | -20.8332 | -21.3709 | -22.0573 | -22.8851 | -23.8495 | -24.9472 | -26.1757 | -27.5333 |
| $E_{\mathrm{HX}}$ | 13.5945 | 15.5612 | 17.4468 | 19.2723 | 21.0520 | 22.7959 | 24.5113 | 26.2033 |
| $E_{\mathrm{X}}$ | -19.7658 | -20.1821 | -20.7984 | -21.5938 | -22.5541 | -23.6692 | -24.9319 | -26.3369 |
| $E_{\mathrm{C}}$ | -1.0673 | -1.1889 | -1.2590 | -1.2913 | -1.2954 | -1.2780 | -1.2438 | -1.1963 |
| $T_{\mathrm{C}}$ | 0.6289 | 0.7457 | 0.8330 | 0.8980 | 0.9453 | 0.9785 | 0.9998 | 1.0112 |
| $T_{\mathrm{C}}^{\mathrm{virial}}$ | 0.6232 | 0.7399 | 0.8270 | 0.8918 | 0.9390 | 0.9719 | 0.9931 | 1.0043 |
| $V_{\mathrm{C}}$ | -1.6962 | -1.9346 | -2.0920 | -2.1893 | -2.2408 | -2.2564 | -2.2436 | -2.2075 |

TABLE VIII. First excitation energy and energy components of He. All the energies are in eV. Exact first excitation energy $E_1 - E_0 = 19.8231$ eV. $T = -E$ according to the virial theorem for atoms. $E_{\mathrm{H}}$ is defined using the traditional definition given in the main text. $T_{\mathrm{C}}^{\mathrm{virial}}$ is obtained by the virial theorem derived in this work.

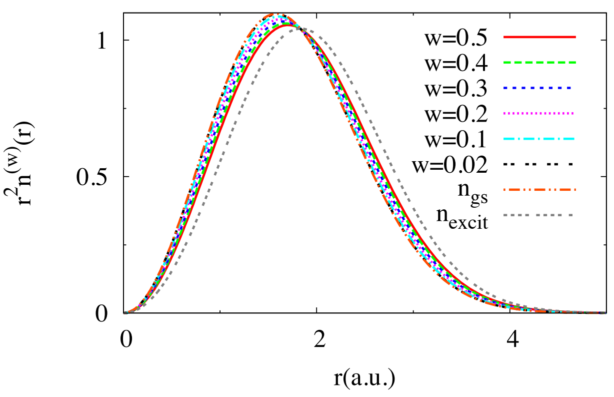


FIG. 3. Exact ensemble radial densities $[r^2 n^{(\mathtt{w})}(r)]$ of the Hooke's atom.

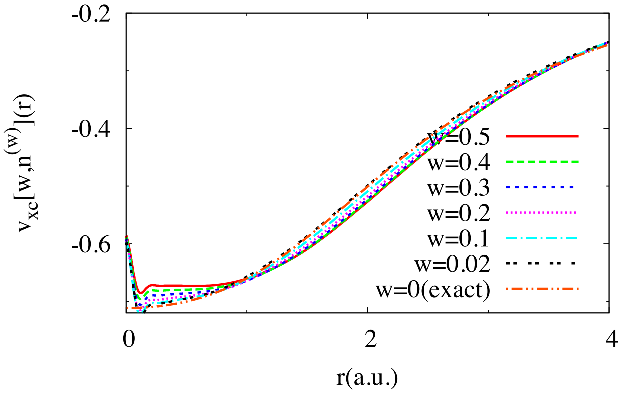


FIG. 4. Exact ensemble xc potentials of the Hooke's atom, with additive constants adjusted to align the potential curves.

### D. Triplet helium ensemble

The triplet ensemble provides an alternative symmetry-projected ensemble to test. The energies of the 1s2s and 1s3s triplet states are

$$E_0^{\mathrm{triplet}} = -59.1902\,\mathrm{eV},$$
$$E_1^{\mathrm{triplet}} = -56.2911\,\mathrm{eV}.$$

Fig. 9 shows that even the exchange-correlation potential corresponding to the largest w-value retains the shape of

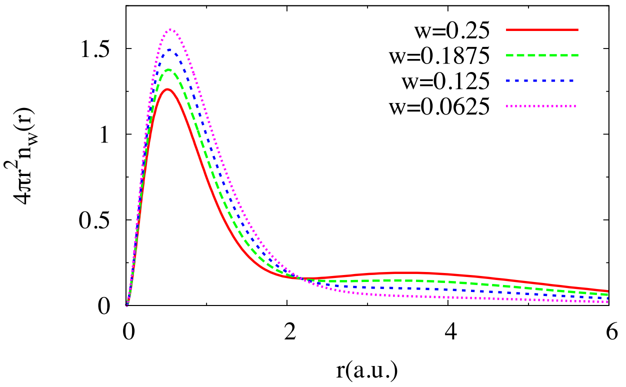


FIG. 5. Ensemble densities of the two-multiplet ensemble of He.

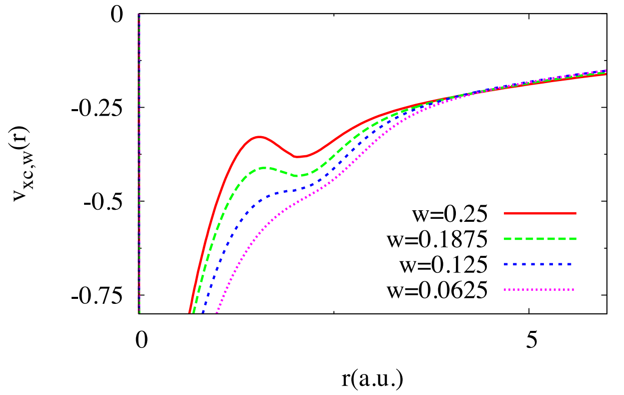


FIG. 6. Ensemble xc potentials of the two-multiplet ensemble of He.

those of smaller w-values. In this way, this set of potentials is similar to that of the 2-multiplet ensemble, and not to that of the singlet ensemble, where higher values of w generate smoother potentials than lower values. As was seen with the singlet ensemble, excitation energies for the triplet-triplet transition that are extracted from the symmetry-projected ensemble are highly accurate (Table IX).

### E. Unambiguous energy density

Virial energy densities are known to have erratic behaviors in ground-state DFT for molecules and solids. As a complement to the virial energy density presented in the main text, we can also define an unambiguous energy density. Mirroring the ground-state case[2], an unambiguous energy density for $E_{\rm HXC}+T_{\rm C}$ is

$$e^{\rm unamb}_{\rm HXC,w}(\mathbf{r})+t^{\rm unamb}_{\rm c,w}(\mathbf{r}) = -\frac{3}{4\pi}\int d^3r'\,\frac{\nabla\cdot[n_{\tt w}(\mathbf{r}')\nabla v_{\rm XC,w}(\mathbf{r}')]}{|\mathbf{r}-\mathbf{r}'|}. \tag{7}$$

Fig. 10 shows the energy densities of $E_{\rm XC}+T_{\rm C}$ defined in the body of our paper as the virial energy density and

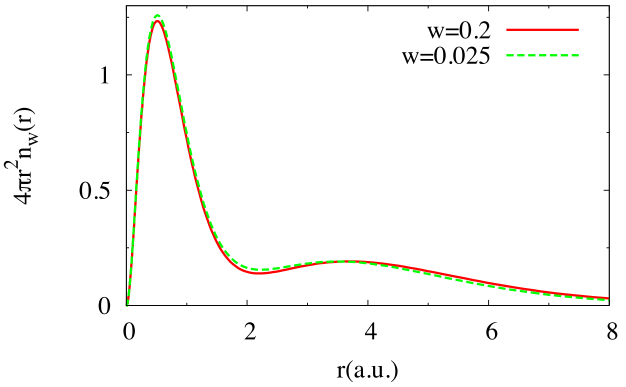


FIG. 7. Ensemble densities of the three-multiplet ensemble of He.

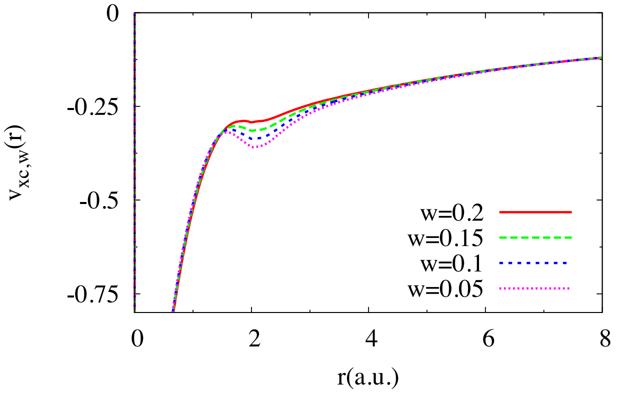


FIG. 8. Ensemble xc potentials of the three-multiplet ensemble of He.

Eq. (7) for $\mathtt{w}=0.5$ helium singlet ensemble. The unambiguous energy density is noticeably smoother than the virial energy density, which shows characteristic bumps that develop as w increases to its maximum value.

[1] M. S. Pindzola, T. W. Gorczyca, and C. Bottcher. Two-photon ionization of lithium in the time-dependent hartree-fock approximation. *Phys. Rev. A*, 47:4982, 1993.
[2] K. Burke, F. G. Cruz, and K.-C. Lam. Unambiguous exchange-correlation energy density for hooke's atom. *Int. J. Quant. Chem.*, 70:583, 1998.

| w | 0.166666 | 0.145833 | 0.125 | 0.104166 | 0.083333 | 0.0625 | 0.041666 | 0.020833 |
|---|---|---|---|---|---|---|---|---|
| $E_1^{\mathrm{KS}} - E_0^{\mathrm{KS}}$ | 2.8928 | 2.8939 | 2.8946 | 2.8952 | 2.8956 | 2.8959 | 2.8963 | 2.8967 |
| $\partial E_{\mathrm{xc,w}}[n]/\partial w\|_{n=n_{\mathtt{w}}}$ | 0.0187 | 0.0151 | 0.0128 | 0.0112 | 0.0104 | 0.0098 | 0.0089 | 0.0074 |
| $(E_1 - E_0)_{\mathtt{w}}$ | 2.8990 | 2.8989 | 2.8989 | 2.8989 | 2.8990 | 2.8992 | 2.8993 | 2.8992 |
| $E_{\mathtt{w}}$ | -57.7406 | -57.9218 | -58.1030 | -58.2842 | -58.4654 | -58.6466 | -58.8278 | -59.0090 |
| $T_{\mathrm{S}}$ | 57.7065 | 57.8862 | 58.0660 | 58.2457 | 58.4255 | 58.6053 | 58.7851 | 58.9649 |
| $E_{\mathrm{H}}$ | 24.2342 | 24.6239 | 25.0221 | 25.4287 | 25.8437 | 26.2671 | 26.6989 | 27.1392 |
| $V$ | -120.718 | -121.337 | -121.956 | -122.575 | -123.194 | -123.813 | -124.432 | -125.051 |
| $E_{\mathrm{XC}}$ | -18.9630 | -19.0947 | -19.2349 | -19.3835 | -19.5405 | -19.7060 | -19.8799 | -20.0622 |
| $E_{\mathrm{HX}}$ | 5.4735 | 5.7475 | 6.0214 | 6.2954 | 6.5694 | 6.8435 | 7.1176 | 7.3918 |
| $E_{\mathrm{X}}$ | -18.7606 | -18.8765 | -19.0007 | -19.1333 | -19.2743 | -19.4236 | -19.5813 | -19.7474 |
| $E_{\mathrm{C}}$ | -0.2024 | -0.2183 | -0.2342 | -0.2502 | -0.2663 | -0.2824 | -0.2986 | -0.3148 |
| $T_{\mathrm{C}}$ | 0.0341 | 0.0356 | 0.0371 | 0.0385 | 0.0399 | 0.0413 | 0.0427 | 0.0441 |
| $T_{\mathrm{C}}^{\mathrm{virial}}$ | 0.0290 | 0.0304 | 0.0319 | 0.0333 | 0.0348 | 0.0361 | 0.0375 | 0.0389 |
| $V_{\mathrm{C}}$ | -0.2365 | -0.2539 | -0.2713 | -0.2887 | -0.3062 | -0.3237 | -0.3413 | -0.3589 |

TABLE IX. First excitation energy and energy components of the triplet ensemble of helium atom. All the energies are in eV. Exact first excitation energy $E_1 - E_0 = 2.8991$ eV. $T = -E$ according to the virial theorem for atoms. $E_{\mathrm{H}}$ is defined in Eq. (29). $T_{\mathrm{C}}^{\mathrm{virial}}$ is obtained by the virial theorem Eq. (62).

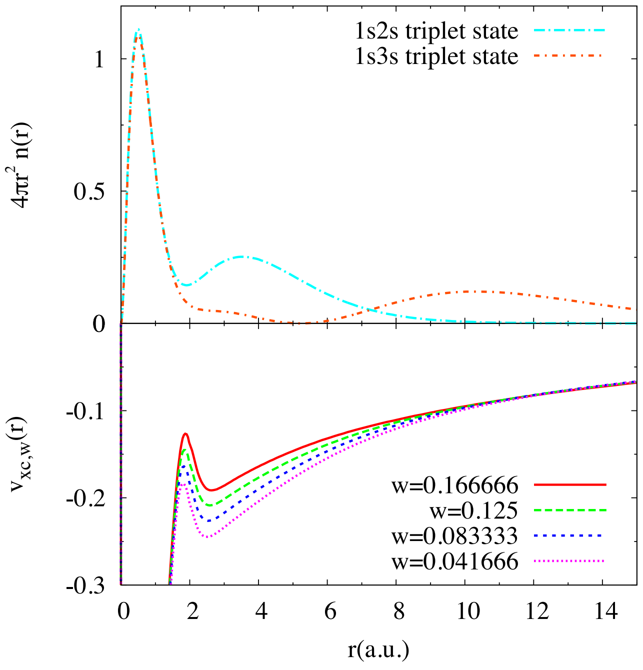


FIG. 9. Exact densities and ensemble xc potentials for a triplet ensemble of He.

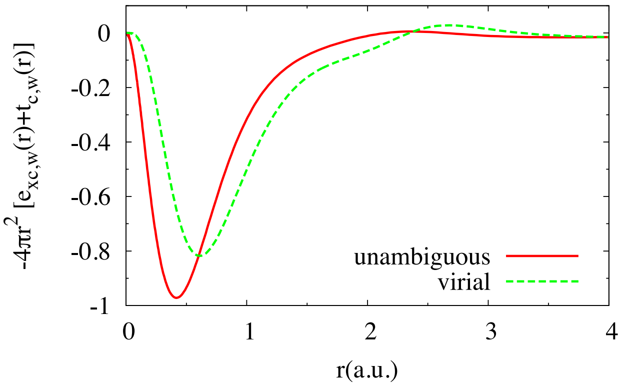


FIG. 10. Comparison of the virial energy density and unambiguous energy density for the singlet ensemble of He at $\mathtt{w} = 0.5$.
